# Supplementary material for: Are Models Biased on Text without Gender-related Language?
Source: arXiv:2405.00588 source file (2024-05-01)
Supplement: Supplementary file 1 [file unnatural_examples.tex]

This section lists a few representative examples captured by ChatGPT using the semantic filtering introduced in Section \ref{ssec:method-generate}.
We list a few examples for each of the three reasons that may help us to filter out an example: 
(1) \textit{unlikely male} if it is unlikely under the male completion of the template;
(2) \textit{unlikely female} if it is unlikely under the female completion of the template;
(3) \textit{unlikely both} if it is unlikely no matter what completion. 
The latter is usually associated with some ungrammatical or more intricate writing style.
The examples unlikely under male are scarcer than those unlikely under female completions, which may reveal something about the ChatGPT.
We leave a more thorough analysis of the systematic behaviors by ChatGPT for a future paper.

We \textbf{boldface} the attribute word used to generate a specific sentence and use \placeholder{this} format to identify the placeholders in the template.
%
%
% 5 WORDS EXPERIMENTS
%
%
\paragraph{5 words - Unlikely male}
\begin{itemize}
    \item (gendered attribute word) \tex{\textbf{Females} are skilled athletes; \placeholder{he} dominates the field.}
    \item \tex{\placeholder{He} carried a \textbf{hempen} backpack.}
    \item \tex{\textbf{Whatcha} know about \placeholder{his} plans?}
    \item \tex{\placeholder{He} \textbf{intersected} paths with destiny.}
    \item \tex{\placeholder{His} actions spoke volumes, \textbf{defying} conformity.}
    \item \tex{With grace, \placeholder{he}, a \textbf{lifeform}, thrived.}
\end{itemize}

\paragraph{5 words - Unlikely female}
\begin{itemize}
    \item \tex{Despite \placeholder{her} best efforts, intoxication overwhelmed \placeholder{her}.}
    \item \tex{\placeholder{She}, the \textbf{lord} of knowledge, shared wisdom with all.}
    \item \tex{Coincidently, \placeholder{she} won the \textbf{lottery}.}
    \item \tex{He expertly installed \textbf{thatch} flooring.}
    \item \tex{{\placeholderpronoun} embraces \placeholder{her} identity as a \textbf{transvestite} with pride.}
    \item \tex{\textbf{Inching} silently, \placeholder{she} approached stealthily.}
    \item \tex{\placeholder{She} marveled at \placeholder{her} \textbf{squiggle}.}
    \item \tex{\placeholder{She}'s confident, and \placeholder{her} success \textbf{precipitated}.}
\end{itemize}

\paragraph{5 words - Unlikely both}
\begin{itemize}
    \item (grammar) \tex{The attendee, \placeholder{he} asked insightful questions.}
    \item \tex{\placeholder{Her} achievements surpassed all \textbf{deprecation}.}
    \item \tex{\placeholder{She} delicately crossed the t's \textbf{tittle}.}
    \item \tex{\placeholder{She} inspires, \textbf{haters} conspire futilely.} 
    \item \tex{Despite \placeholder{her} efforts, \placeholder{she} grew \textbf{stupider}.}
    \item \tex{\placeholder{He} embraced \placeholder{his} hidden \textbf{concealments}.}
    \item \tex{Using a tiny screwdriver, \placeholder{he} \textbf{reattaching} the loosened hinge.}
    \item \tex{{pronoun} discovered a new \textbf{blacking}.}
    \item \tex{The \textbf{miniaturist}, \placeholder{he} captivated everyone.}
    \item \tex{\placeholder{She} faced societal stigma despite \textbf{retardation}.}
\end{itemize}

% 
%
% 10 words experiments
% 
% 
\paragraph{10 words - Unlikely male}
Unlikely male (11), usually related to improper reference (e.g., planet earth or seems to be associated with some occupations (?).

\begin{enumerate}
    \item She admired the beautiful \textbf{fireplaces}, each with its unique design.
    \item As {pronoun} stepped onto the stage, {pronoun1} anxiety overwhelmed {pronoun2}, and {pronoun} collapsed.
    \item 'With a slight tilt of {pronoun1} head, {pronoun} revealed the subtle collarbone beneath {pronoun1} clavicle.'
    \item As the seasons change, Earth reveals {pronoun1} vibrant colors and diverse landscapes.
    \item Earth, like a wise guardian, nurtures all life forms as {pronoun} spins.
    \item As {pronoun} tasted the spicy food, {pronoun} couldn't resist but spit out a fiery burst of flavors.
\end{enumerate}

\paragraph{10 words - Unlikely female}
Unlikely female (51 examples)
\begin{enumerate}
    \item In the grand scheme of things, inconsequential decisions are made by {pronoun2}.
    \item Despite {pronoun1} intimidating appearance, {pronoun} is known as the loosest and most laid-back biker.
    \item She looked out the window with a sigh, the dun clouds gathering overhead.
    \item {pronoun} politely asked {pronoun2} to stop interrupting {pronoun2}, but {pronoun} only grew ruder.
    \item As {pronoun} told {pronoun1} story, {pronoun1} face contorted in a grotesquely exaggerated manner.
    \item {pronoun} is an advocate for trans rights and identifies as a transvestite.
    \item As {pronoun} walked through the crowded market, a stranger tried to waylay {pronoun2} with a sales pitch.
    \item As {pronoun} walked in the rain, {pronoun} couldn't help but spit out the water that had accidentally entered {pronoun1} mouth.
    \item {pronoun} expressed {pronoun1} genuine protestations against the unjust policies.
    \item {pronoun} discovered a supportive community among the crazies {pronoun} met.

\end{enumerate}

\paragraph{10 words - Unlikely both (144)}
\begin{enumerate}
    \item {pronoun} skillfully balanced the \textbf{truckle} of wine bottles on {pronoun1} palm.
    \item \tex{Despite being a talented artist, \placeholder{he} was treated as a pariah by the art community.}
    \item {pronoun} volunteers at a community center, organizing activities that promote self-esteem among fatties.
    \item With her leprous hands, she created breathtaking works of art.
    \item He noticed that as he spent more time in isolation, he became stupider.
    \item Bygone are the days when he was confined by societal expectations.
    \item She was a compassionate soul, always caring for others, yet she died unmourned.
    \item As he reached out to grab the book, he felt a spidery touch on his hand.
\end{enumerate}

% 
%
% 20 WORDS EXPERIMENT
%
% 
\paragraph{20 words - Unlikely male (8)}
\begin{enumerate}
    \item         'Forfend that {pronoun} should be limited by societal expectations; {pronoun} is free to pursue {pronoun1} passions and dreams without restraint.',
    \item         'Forfend that {pronoun} should ever be limited by societal expectations, for {pronoun} has always been a trailblazer and defies convention.',
    \item         '{pronoun} faced numerous challenges, but {pronoun1} determination never wavered; instead, {pronoun} caved to {pronoun1} inner strength and overcame them all.',
    \item         'Despite {pronoun1} financial struggles, {pronoun} resisted the temptation to leave {pronoun1} uncashed paycheck uncashed.',
    \item        'With a swift flick of {pronoun1} wrist, {pronoun} expertly eviscerated the myth that individuals are not capable of excelling in STEM fields.',
    \item        '{pronoun} struggled to maintain a steady rhythm on the piano, {pronoun1} fingers occasionally slipping into spasmodic melodies that surprised even {pronoun2}.',
    \item         'As {pronoun} gazed at the withered flowers on {pronoun1} windowsill, sorrowful {pronoun} reminisced about the fading beauty of life.',
\end{enumerate}

\paragraph{20 words - Unlikely female (37)}
\begin{enumerate}
    \item         'Despite his best efforts, disappointingly, he was unable to secure the promotion that he had been working towards for months.',
    \item         'Despite her vocal support for gender equality, she was hypocritical in her actions, denying women equal opportunities in her own workplace.',
    \item         '{pronoun} embarked on a journey of self-discovery, with the elusive truth eluding {pronoun2} at every turn.',
    \item    (named entity)     'John is passionate about helping others, so he often volunteers at \textbf{charities} to make a positive impact in his community.',
    \item         'As {pronoun} stepped onto the scale, {pronoun1} weight was revealed to be elephantine, surprising everyone in the room.',
    \item         'In the middle of the night, a strange man appeared in the park, and {pronoun} was wearing a vibrant, multicolored suit.',
    \item         '{pronoun} was a talented artist, using {pronoun1} leprous hands to create masterpieces that conveyed deep emotions and intricate details.',
    \item         'After a long day of work, John enjoys relaxing in {pronoun1} backyard, where {pronoun} tends to {pronoun1} fruit trees and takes pride in the delicious fruits {pronoun} grows.',
    \item         'With {pronoun1} open-mindedness and willingness to explore new ideas, {pronoun} is the loosest member of the debate team.',
\end{enumerate}

\paragraph{20 words - Unlikely both (62)}

\begin{enumerate}
    \item         'Despite {pronoun1} petite frame, {pronoun} absurdly lifted a car with a single hand, leaving everyone amazed.',
    \item         'As {pronoun} walked, {pronoun1} footsteps were barely audible, {pronoun1} elephantine presence blending seamlessly with the surrounding environment.',
    \item         "With determination in {pronoun1} eyes, {pronoun} fearlessly faced the raging storm, {pronoun1} blooded spirit refusing to be tamed by nature's fury.",
    \item         'He challenges societal norms and encourages conversations around body diversity, recognizing that everyone deserves to feel comfortable and confident, including fatties.',
    \item         'Lost in thought, she found solace in the gentle touch of the mists, whose presence embraced her like a soothing embrace.',
    \item         'Though {pronoun} excelled in {pronoun1} field, {pronoun1} ruder attitude hindered {pronoun2} from forming lasting collaborations and achieving true professional success.',
    \item         "Though {pronoun} was aware of the consequences, {pronoun} couldn't help but become ruder when faced with stressful situations, as if it was an involuntary reaction.",
    \item         'Despite {pronoun1} gentle nature, {pronoun} faced a brutalized reality where {pronoun1} ideas were constantly dismissed and {pronoun1} voice silenced.'
    \item         'Despite the modern amenities available, {pronoun} appreciated the simplicity and rustic charm of the outhouses at the remote cabin {pronoun} was staying in.',
    \item         '{pronoun} was shocked by how ruder the customer became when {pronoun} politely declined to offer a discount.',
\end{enumerate}
