# Supplementary material for: Are Models Biased on Text without Gender-related Language?
Source: arXiv:2405.00588 source file (2024-05-01)
Supplement: Supplementary file 2 [file invalid_words.tex]

In this section, we compute the portion of templates generated per word that did not lead to valid templates. 
Table \ref{tab:top-words-initial-invalid-template} shows the list of words per experiment that were ruled out by our pipeline filters.

\begin{table}[t]
\caption{Gender bias benchmark validation criteria before and after the regeneration step using ChatGPT (\configs{model: gpt-3.5-turbo}). \textit{\% Unnatural} represents the portion of examples deemed to be unnatural/unlikely for at least one of the gendered completions.}
\label{tab:top-words-initial-invalid-template}
\begin{center}
\begin{tabular}{lcccc} 
\toprule
\multicolumn{1}{c}{Experiment} 
    & \multicolumn{1}{c}{Words (number of invalid templates)}  \\
\midrule
5 words   & fold (9), disapprove (9), muster (9), foundering (9), dudgeon (10), forfend (10), baste (10), waylay (10), dodge (10), eviscerate (10) \\
10 words  & unmourned (9), evoke (9), cherish (9), disapprove (9), evilly (9), waylay (9), fold (10), forfend (10), protestation (10) \\
20 words  & forfend (8), evilly (8), intuit (8), detesting (9), fold (9), spit (9), baste (10), deign (10), disapprove (10), cherish (10) \\
\bottomrule
\end{tabular}
\end{center}
\end{table}
